# Supplementary material for: SSAP: A Shape-Sensitive Adversarial Patch for Comprehensive Disruption of Monocular Depth Estimation in Autonomous Navigation Applications
Source: arXiv:2403.11515 source file (2024-08-05)
Supplement: Supplementary file 1 [file suplementary.tex]

\begin{figure}[!ht]
\centering
\includegraphics[width=\columnwidth]{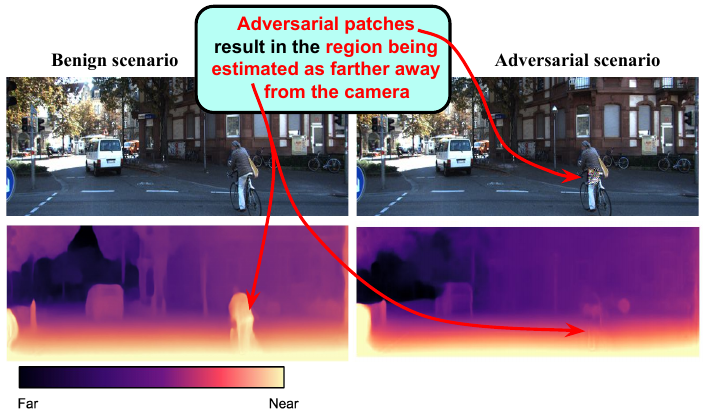}
\caption{Impact of SSAP on pedestrian/cyclist class for CNN-based MDE. The cyclist seamlessly blends with the background.}
\label{results_ped}
\end{figure}
